# Supplementary material for: Evolving spatiotemporal patterns and urban scaling of deaths from external causes
Source: arXiv:2601.08754 source file (2026-01-13)
Supplement: Supplementary file 1 [file supplementary.pdf]

# Evolving spatiotemporal patterns and urban scaling of deaths from external causes

**Cesar I. N. Sampaio Filho[1,2], Humberto A. Carmona[1,2], Antonio S. Lima Neto[3,4], Monica V. Prates[5], Haroldo V. Ribeiro[5,*], Marcia C. Castro[6], and José S. Andrade Jr.[1,2,*]**

[1]Departamento de Física, Universidade Federal do Ceará, 60451-970 Fortaleza, Ceará, Brazil
[2]Escola de Saúde Pública do Ceará, 60165-090, Fortaleza, Ceará, Brazil
[3]Laboratório de Ciência de Dados e Inteligência Artificial, Universidade de Fortaleza, Fortaleza, Ceará, Brazil
[4]Secretaria Executiva de Vigilância em Saúde, Secretaria da Saúde do Ceará, Fortaleza, Ceará, Brazil
[5]Departamento de Física, Universidade Estadual de Maringá, Maringá PR 87020-900, Brazil
[6]Department of Global Health and Population, Harvard T. H. Chan School of Public Health, Boston, Massachusetts, USA
[*]email: hvribeiro@uem.br; soares@fisica.ufc.br

## Supplemental Materials

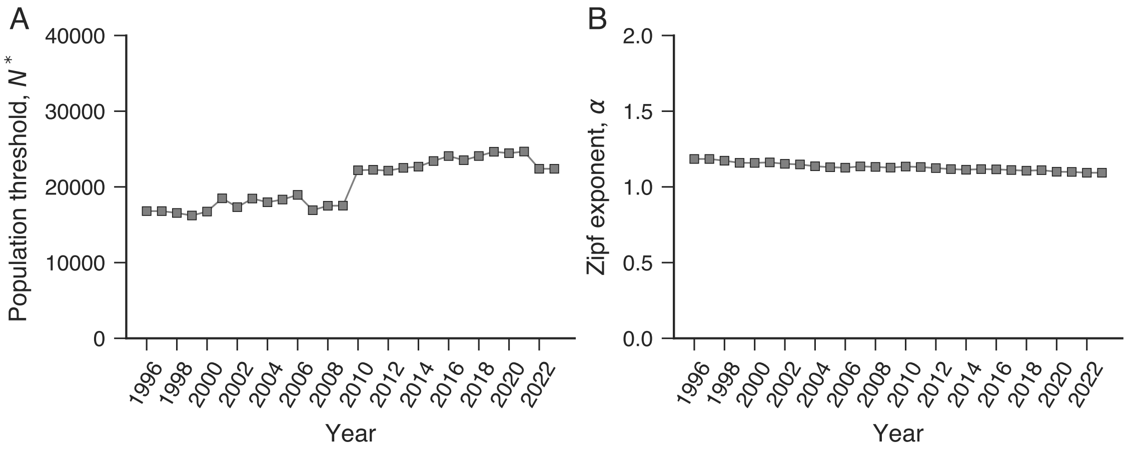


**Figure S1.** Selection of cities based on Zipf's law adherence. (A) The estimated lower bound of the power-law regime of the population distribution $N^*$ and (B) Zipf's law exponent $\alpha$ for Brazilian cities across different years. The values of $N^*$ exhibit fluctuations around 20,000, while the estimated Zipf's law exponents remain close to 1.1 over time. These estimates were obtained using the Clauset-Shalizi-Newman method, which simultaneously determines $\alpha$ and $N^*$ for the population distribution. Only cities with $N \geq N^*$ were included in the scaling analysis to ensure consistency with the assumptions of urban scaling theory.

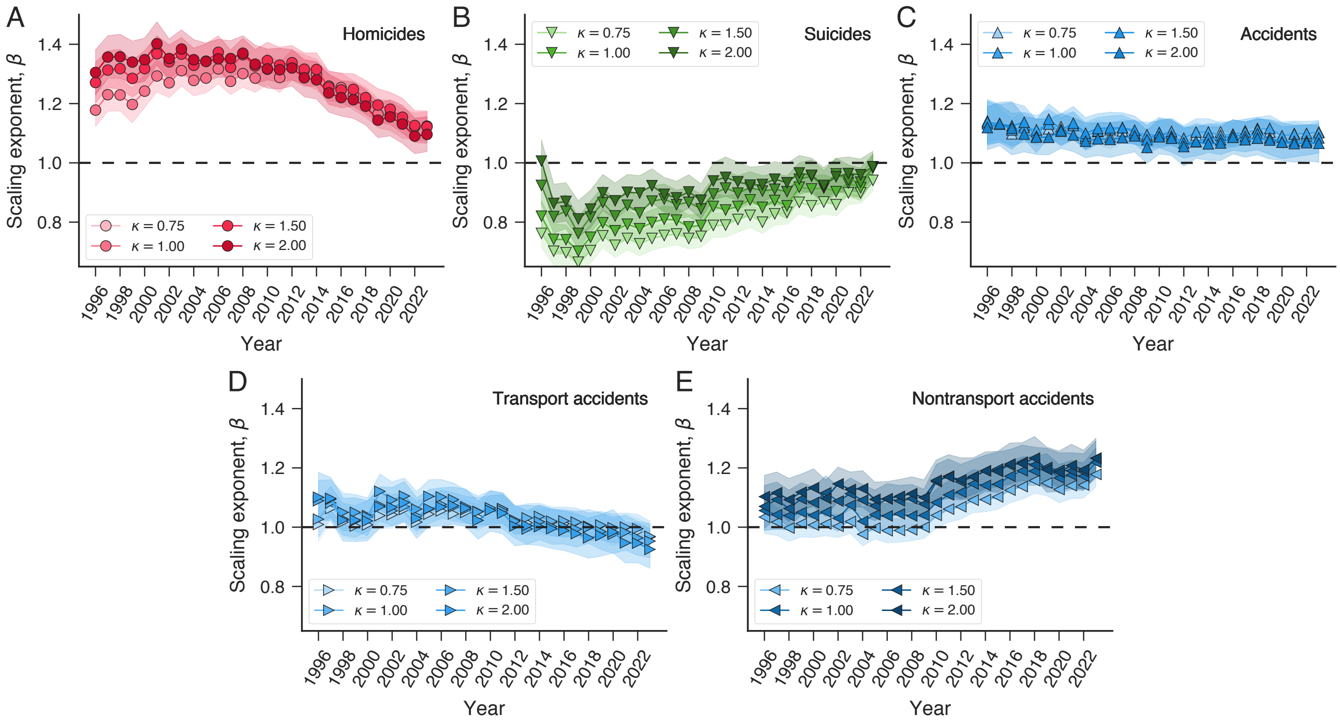


**Figure S2.** Robustness of urban scaling exponents to alternative population thresholds. Estimates of the urban scaling exponents $\beta$ for (A) homicides, (B) suicides, (C) accidents, (D) transport accidents, and (E) nontransport accidents. In each panel, curves show the evolution of $\beta$ obtained from our Bayesian hierarchical model under different population thresholds (represented by varying color shades). Shaded regions represent the 96% highest density (credible) intervals, with dashed lines indicating the isometric scaling regime. For each external cause of death, the color shades indicate estimates obtained for cities with $N \geq \kappa N^*$, where $N$ is population, $N^*$ is the lower bound of the power-law regime of the population distribution, and $\kappa \in (0.75, 1, 1.5, 2)$ tunes the population cutoff ($\kappa = 1$ correspond to the results reported in the main text). The temporal patterns of the scaling exponents are stable across thresholds, indicating that our conclusions are not artifacts of a particular population cutoff inferred from Zipf's law.

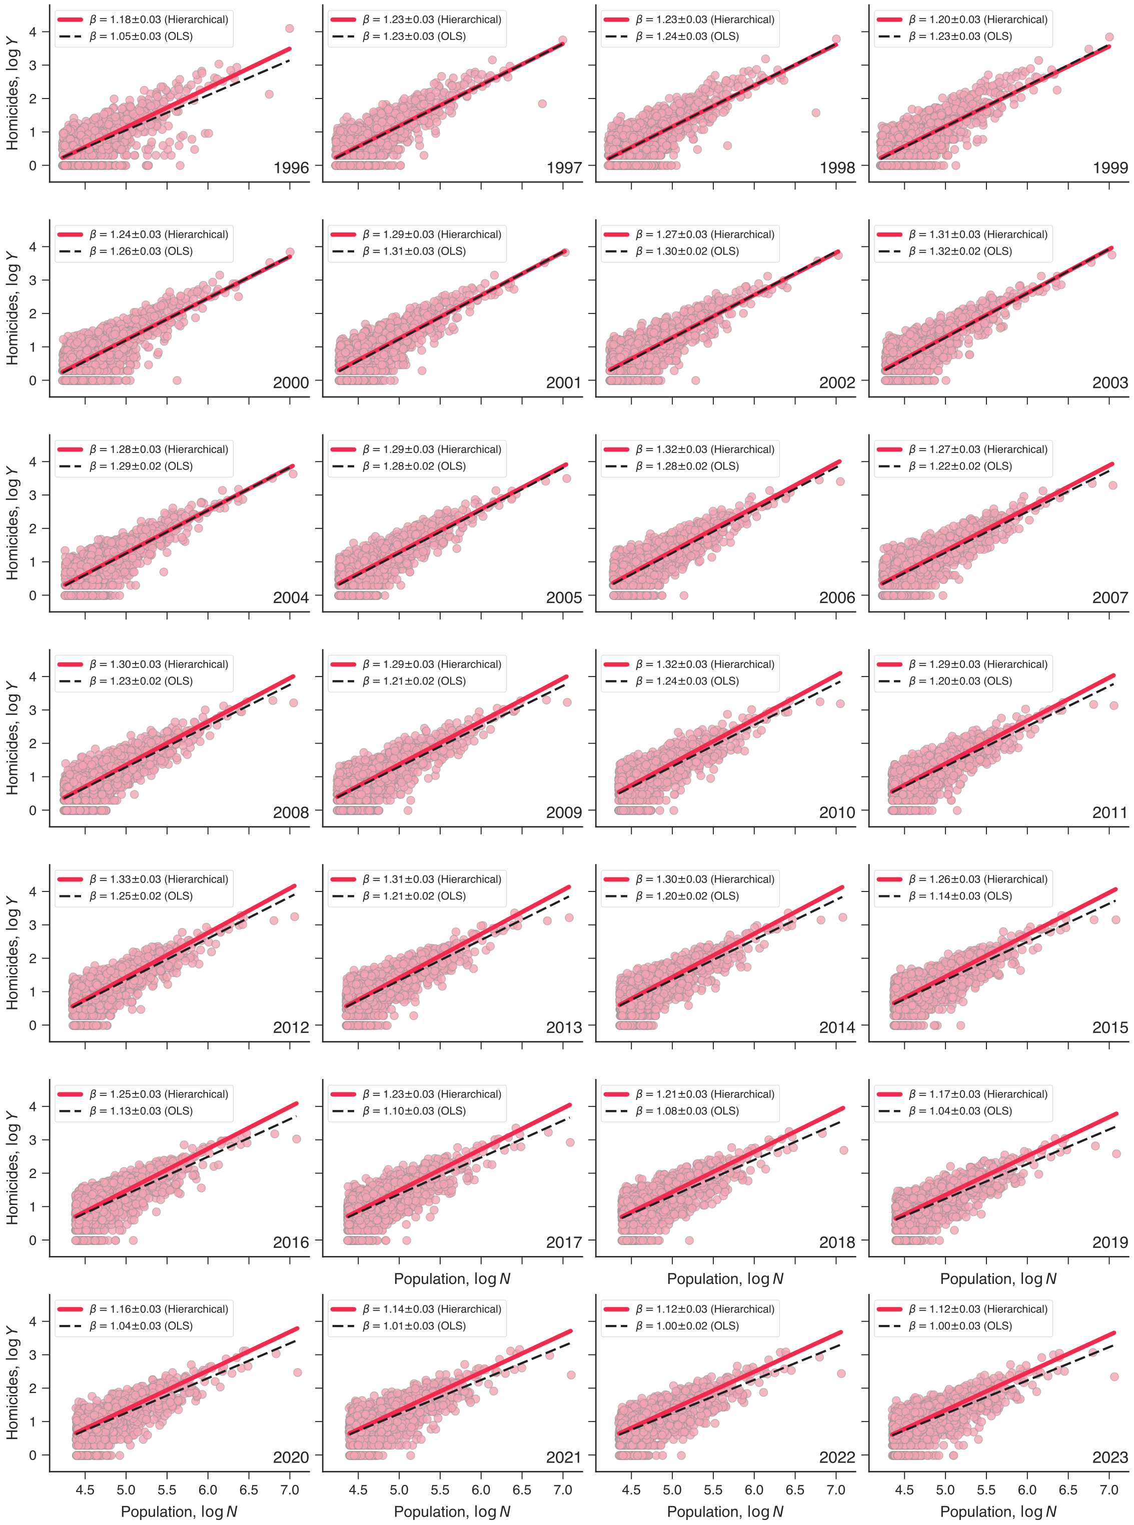


**Figure S3.** Temporal evolution of urban scaling laws for homicides in Brazil. Population scaling relations for homicides across 28 years (1996–2023). Markers represent the number of homicide deaths ($Y$) versus the population ($N$) of Brazilian cities on a base-10 logarithmic scale ($\log Y$ versus $\log N$). Continuous lines indicate the nationwide scaling laws estimated using a Bayesian hierarchical approach, while dashed lines represent scaling laws obtained via the ordinary least-squares (OLS) method applied to log-transformed data. The urban scaling exponents and their standard errors are provided in the plot legends. Over time, the Bayesian estimated scaling exponents remain consistently higher than those obtained via OLS, and a notable decline in the scaling exponent for homicides was observed after 2012, suggesting a weakening of the superlinear effect with population size.

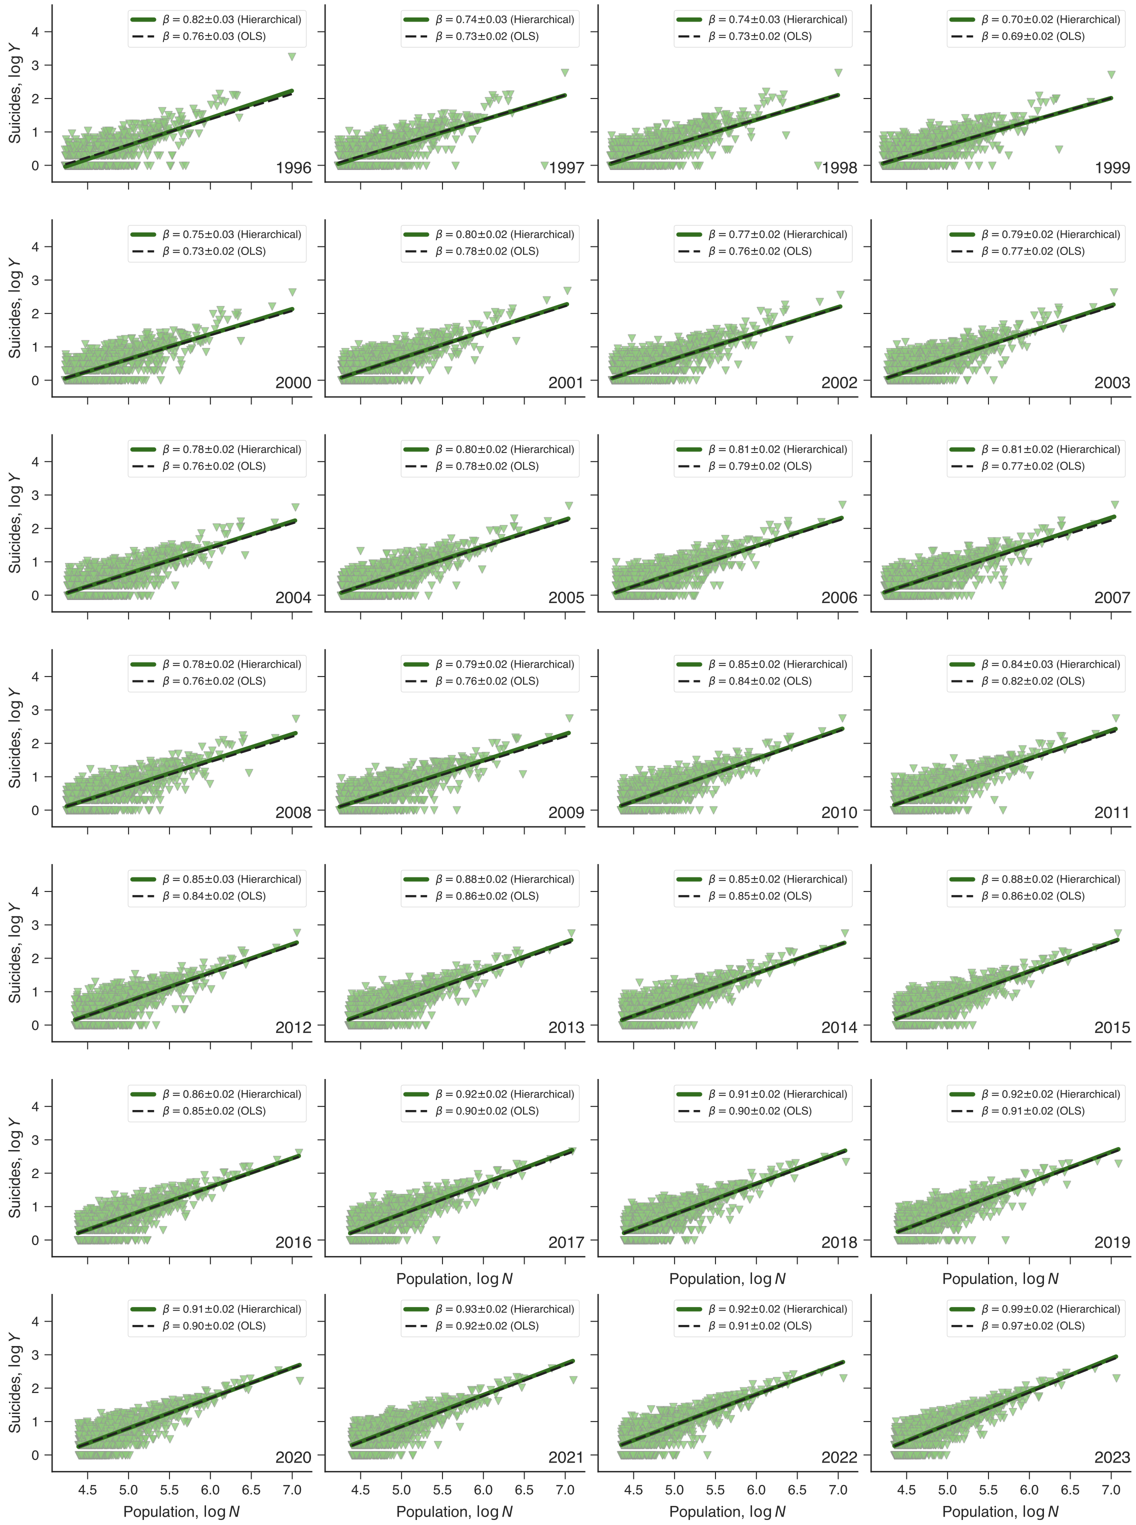


**Figure S4.** Temporal evolution of urban scaling laws for suicides in Brazil. Population scaling relations for suicides across 28 years (1996–2023). Markers represent the number of suicide deaths ($Y$) versus the population ($N$) of Brazilian cities on a base-10 logarithmic scale ($\log Y$ versus $\log N$). Continuous lines indicate the nationwide scaling laws estimated using a Bayesian hierarchical approach, while dashed lines represent scaling laws obtained via the ordinary least-squares (OLS) method applied to log-transformed data. The urban scaling exponents and their standard errors are provided in the plot legends. Over time, the Bayesian estimated scaling exponents remain closely aligned with those obtained via OLS. A gradual increase in the scaling exponent is observed, suggesting a weakening of the sublinear effect with population size.

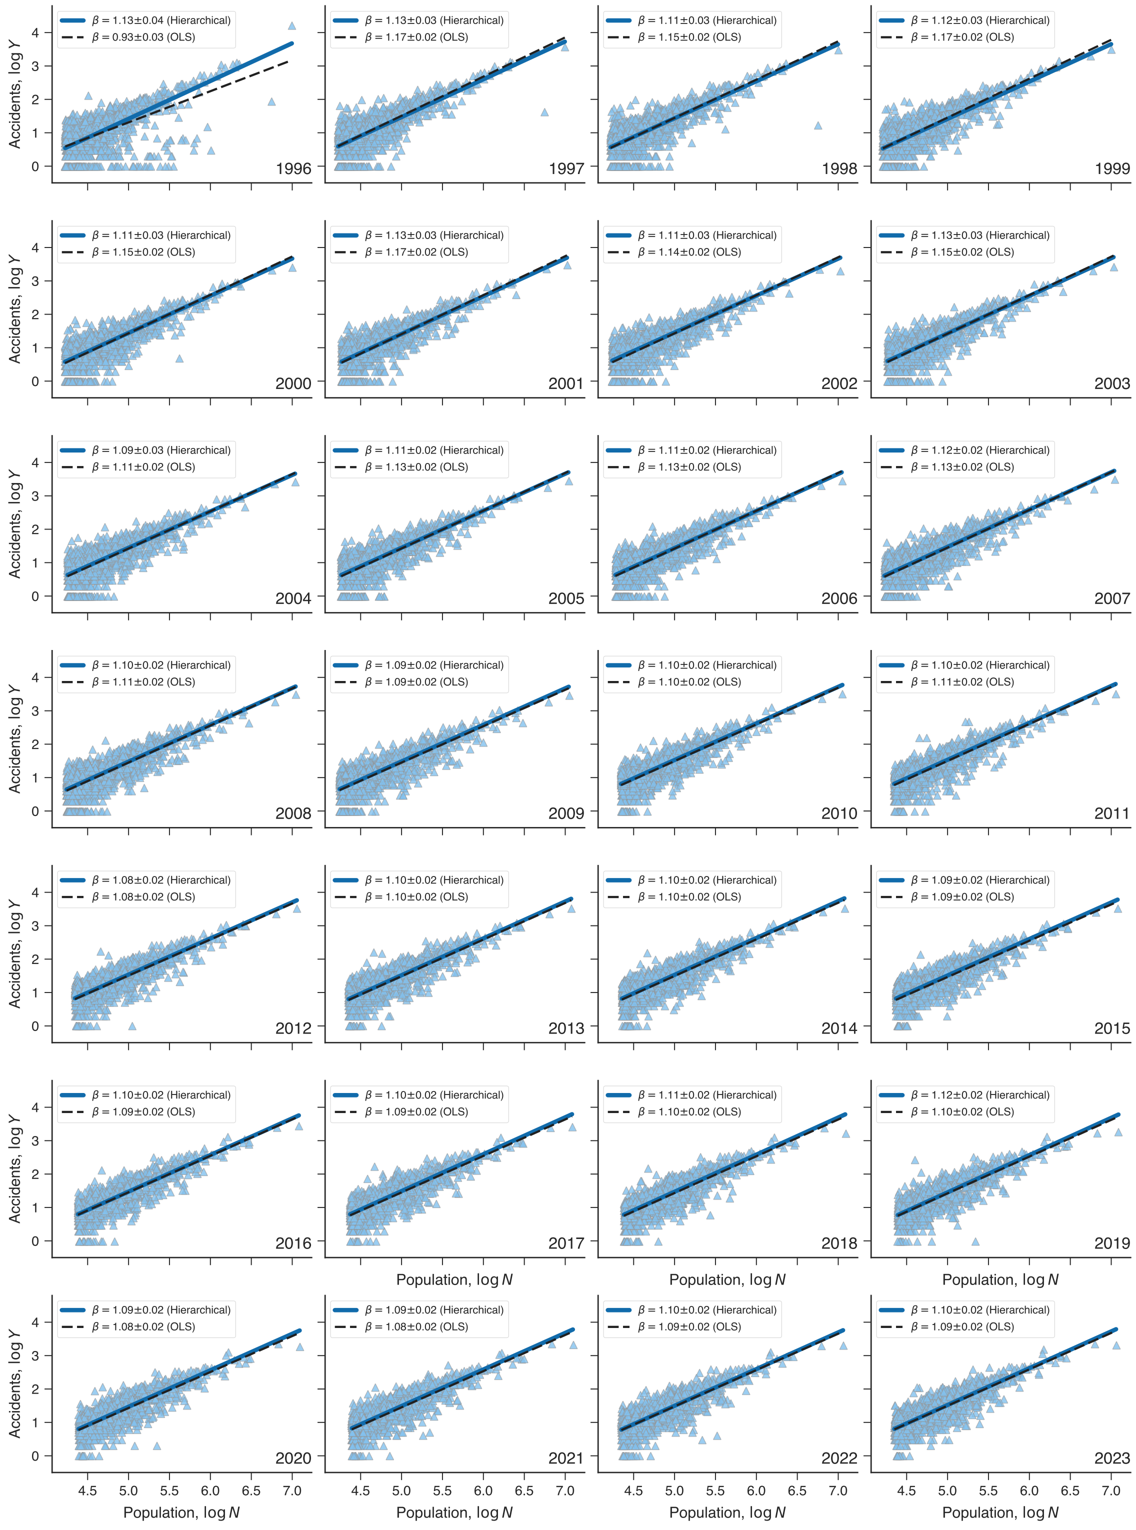


**Figure S5.** Temporal evolution of urban scaling laws for accidents in Brazil. Population scaling relations for accidents across 28 years (1996–2023). Markers represent the number of accident-related deaths ($Y$) versus the population ($N$) of Brazilian cities on a base-10 logarithmic scale ($\log Y$ versus $\log N$). Continuous lines indicate the nationwide scaling laws estimated using a Bayesian hierarchical approach, while dashed lines represent scaling laws obtained via the ordinary least-squares (OLS) method applied to log-transformed data. The urban scaling exponents and their standard errors are provided in the plot legends. The scaling exponent remains stable over time at approximately 1.1, indicating a persistent superlinear relationship.

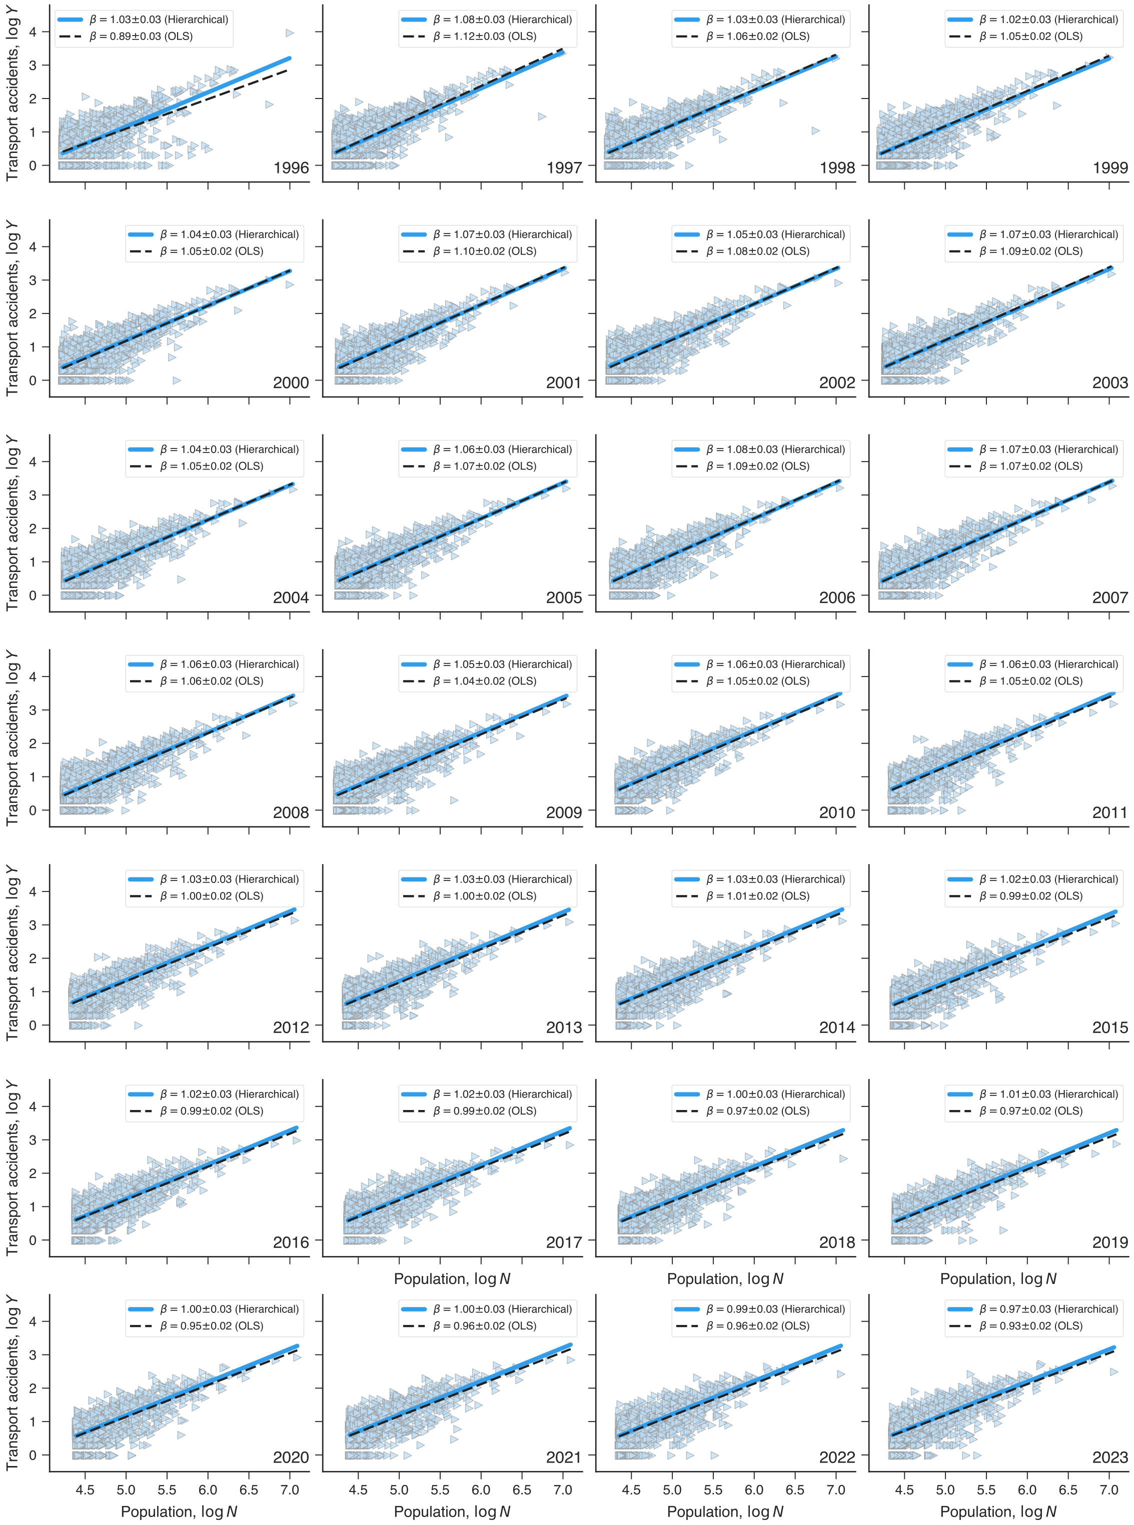


**Figure S6.** Temporal evolution of urban scaling laws for transport accidents in Brazil. Population scaling relations for transport accident-related deaths across 28 years (1996–2023). Markers represent the number of deaths ($Y$) due to transport accidents versus the population ($N$) of Brazilian cities on a base-10 logarithmic scale ($\log Y$ versus $\log N$). Continuous lines indicate the nationwide scaling laws estimated using a Bayesian hierarchical approach, while dashed lines represent scaling laws obtained via the ordinary least-squares (OLS) method applied to log-transformed data. The urban scaling exponents and their standard errors are provided in the plot legends. The scaling exponent remains approximately stable over time and is close to 1, particularly after 2012, indicating a near-linear relationship between transport accident-related deaths and urban population.

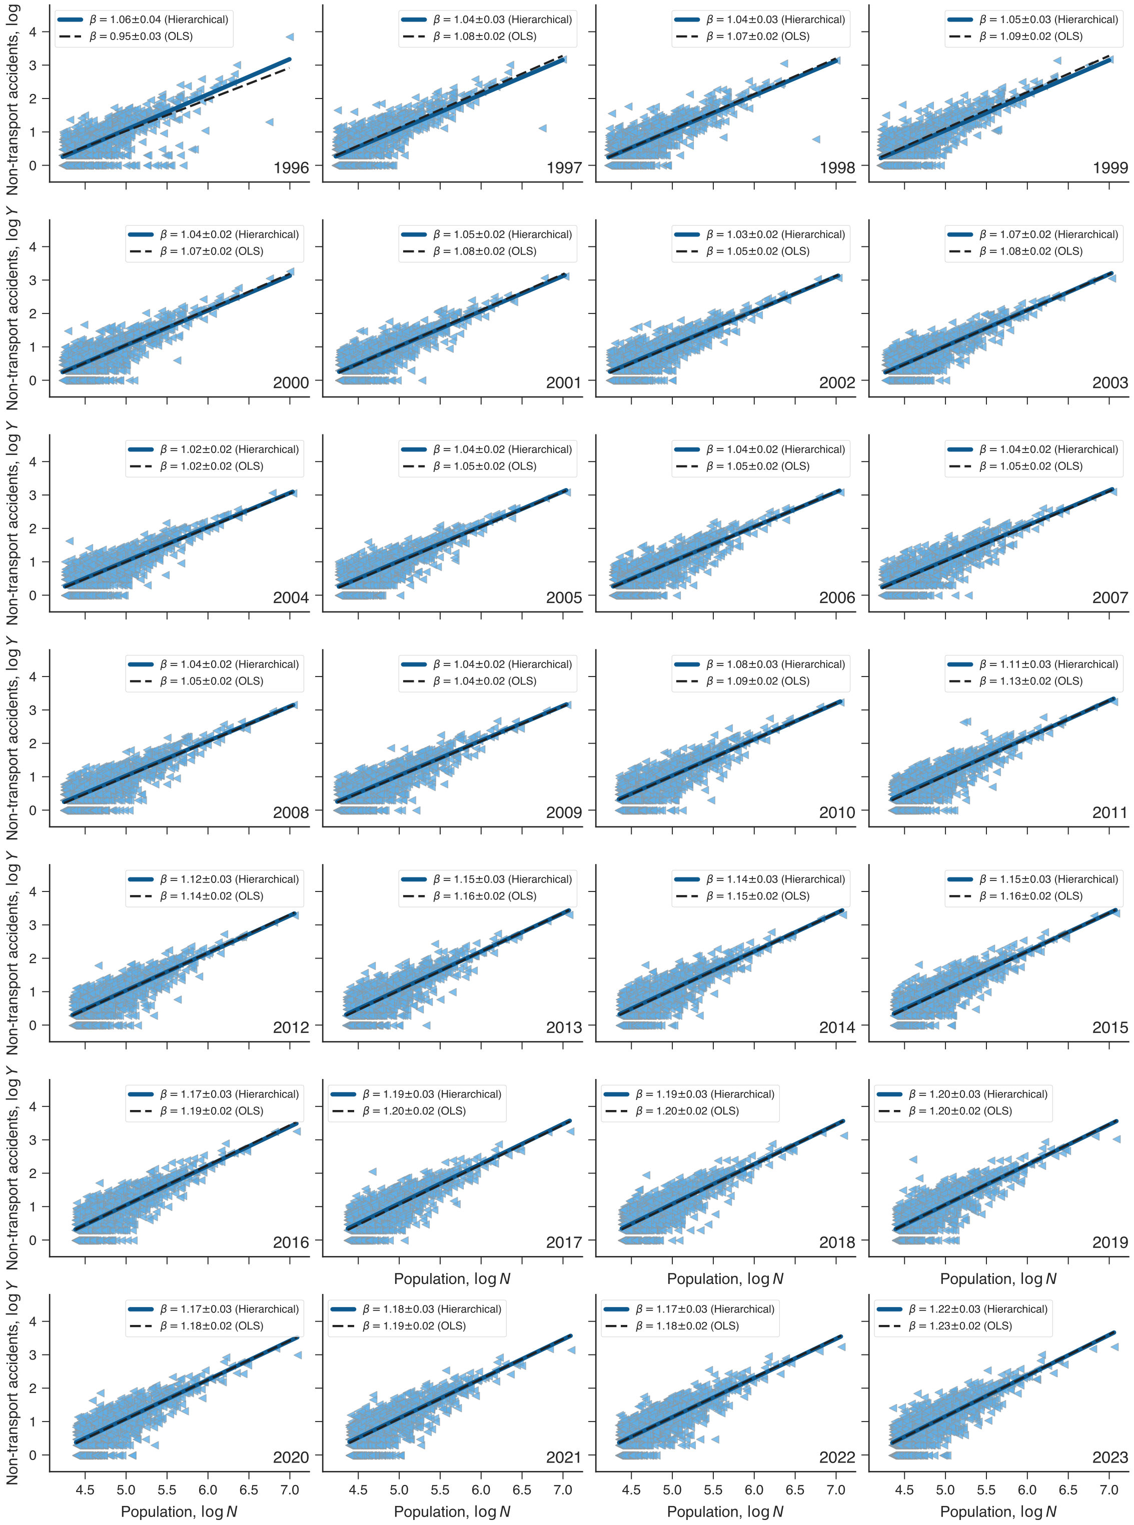


**Figure S7.** Temporal evolution of urban scaling laws for non-transport accidents in Brazil. Population scaling relations for non-transport accident-related deaths across 28 years (1996–2023). Markers represent the number of deaths ($Y$) due to non-transport accidents versus the population ($N$) of Brazilian cities on a base-10 logarithmic scale ($\log Y$ versus $\log N$). Continuous lines indicate the nationwide scaling laws estimated using a Bayesian hierarchical approach, while dashed lines represent scaling laws obtained via the ordinary least-squares (OLS) method applied to log-transformed data. The urban scaling exponents and their standard errors are provided in the plot legends. Before 2010, the scaling exponent remained close to 1, indicating an approximately linear relationship. However, after 2010, the exponent began to increase, becoming superlinear.

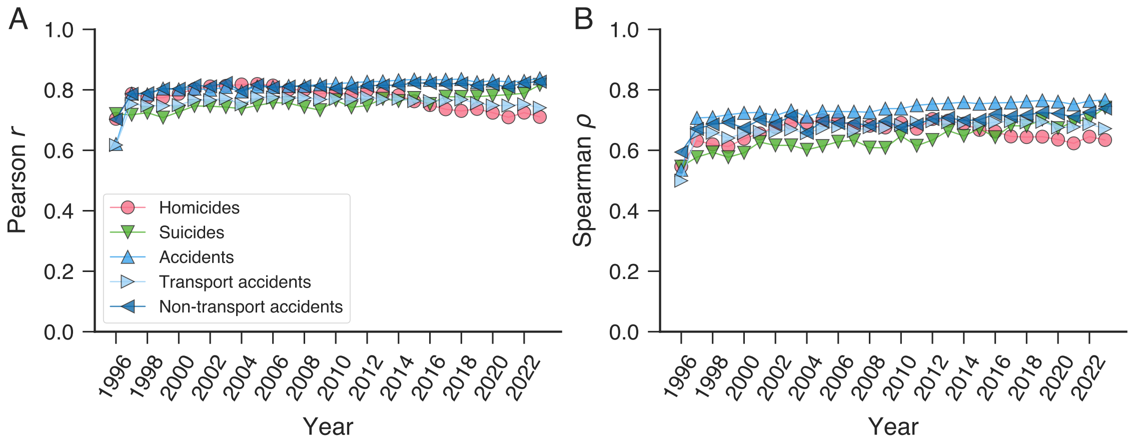


**Figure S8.** Stability of correlation measures for urban scaling relations of external causes of death. (A) Pearson correlation coefficient and (B) Spearman's rank correlation coefficient for the scaling relations of homicides, suicides, accidents, transport accidents, and non-transport accidents across 28 years (1996–2023). Both correlation measures remain approximately stable over time, with Pearson's $r$ fluctuating around 0.8 and Spearman's $\rho$ around 0.7. These results indicate a consistent strength of association between the number of deaths and city population across different external causes of death, reinforcing the robustness of the observed scaling patterns.

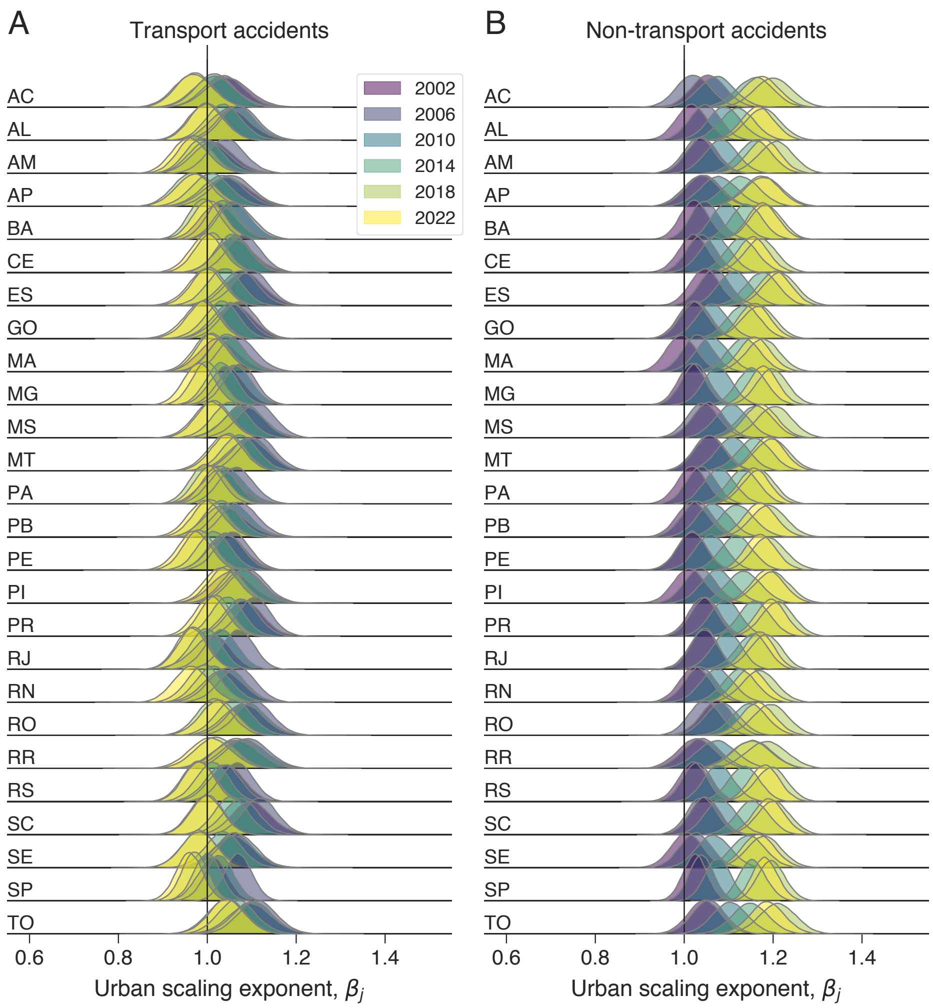


**Figure S9.** Individual evolution of mortality scaling exponents for transport-related and non-transport-related accidents across Brazilian states from 1996 to 2023. Colored curves represent the posterior probability distribution of $\beta_j$ for each $j$, estimated for (A) transport-related accidents and (B) non-transport-related accidents. Each row of plots corresponds to a Brazilian state (denoted by its two-letter abbreviation), with colors indicating different years (as shown in the legend). Vertical lines in both panels denote the isometric regime. The posterior distributions for transport-related accidents remain approximately stationary but exhibit greater variation across states. In contrast, the distributions for non-transport-related accidents shift toward larger values, following national trends, and display less variation across states.

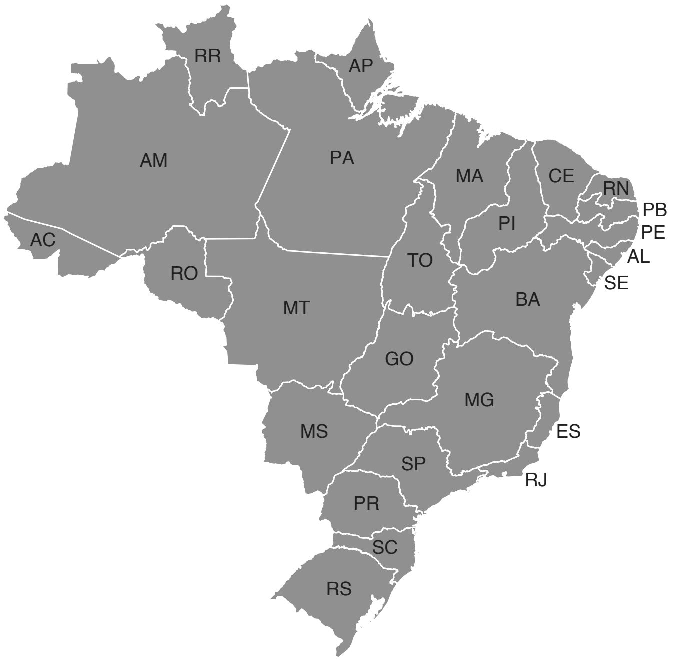


**Figure S10.** Geographical location of Brazilian states. Acronyms by region: North – AC: Acre, AP: Amapá, AM: Amazonas, PA: Pará, RO: Rondônia, RR: Roraima, TO: Tocantins; Northeast – AL: Alagoas, BA: Bahia, CE: Ceará, MA: Maranhão, PB: Paraíba, PE: Pernambuco, PI: Piauí, RN: Rio Grande do Norte, SE: Sergipe; Center-West – GO: Goiás, MT: Mato Grosso, MS: Mato Grosso do Sul; Southeast – ES: Espírito Santo, MG: Minas Gerais, RJ: Rio de Janeiro, SP: São Paulo; South – PR: Paraná, RS: Rio Grande do Sul, SC: Santa Catarina.

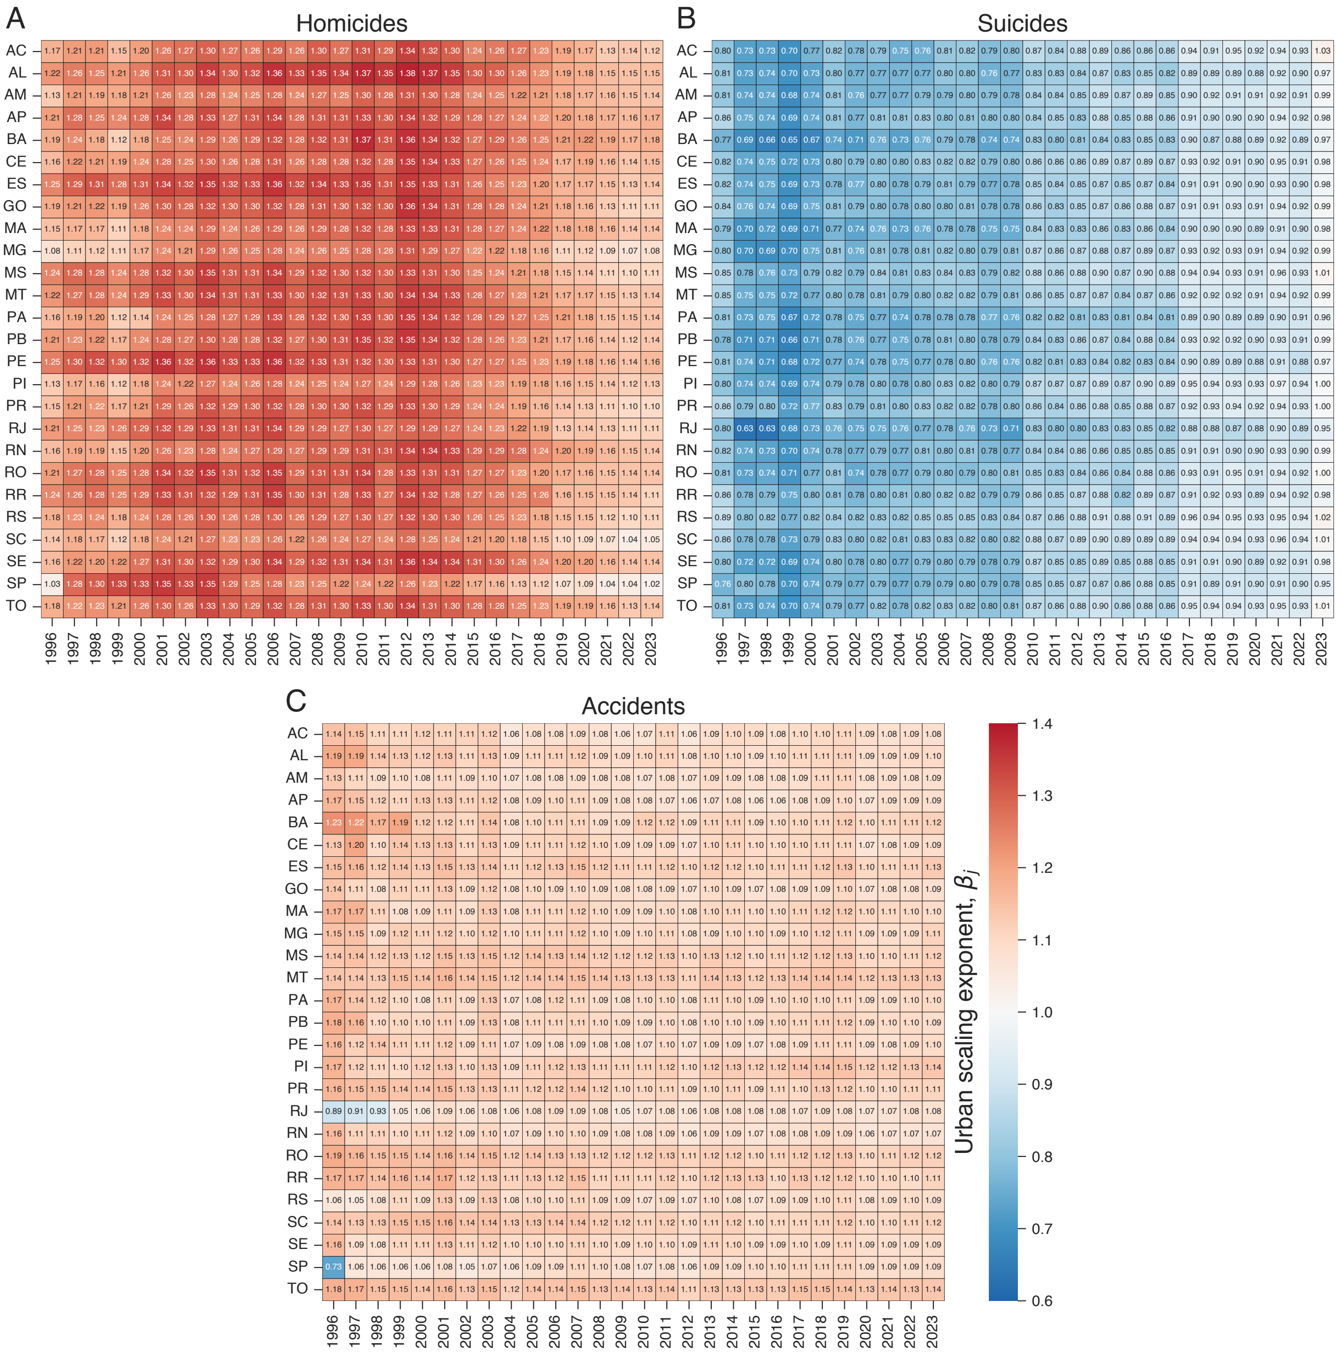


**Figure S11.** Evolution of mortality scaling exponents for each Brazilian state (1996–2023) quantified by point estimates. Matrix plots display the mean of the posterior distribution of $\beta_j$ over the period for each state. Heatmaps are arranged with rows representing states (denoted by their two-letter abbreviations) and columns corresponding to years. Panels show results for (A) homicides, (B) suicides, and (C) accidents, using a uniform color scale in which blueish hues indicate sublinear exponents and reddish hues denote superlinear exponents. These visualizations indicate that the evolution of $\beta_j$ in each state mirrors national trends. Homicide exponents peaked around 2012 before declining, with some states (*e.g.* São Paulo/SP and Santa Catarina/SC) approaching the isometric regime closely, while others (*e.g.* Bahia/BA and Pernambuco/PE) retained higher exponent values. Suicide exponents displayed a uniform shift toward an isometric regime from a sublinear baseline across all states, whereas accident exponents remained stable in a superlinear regime.

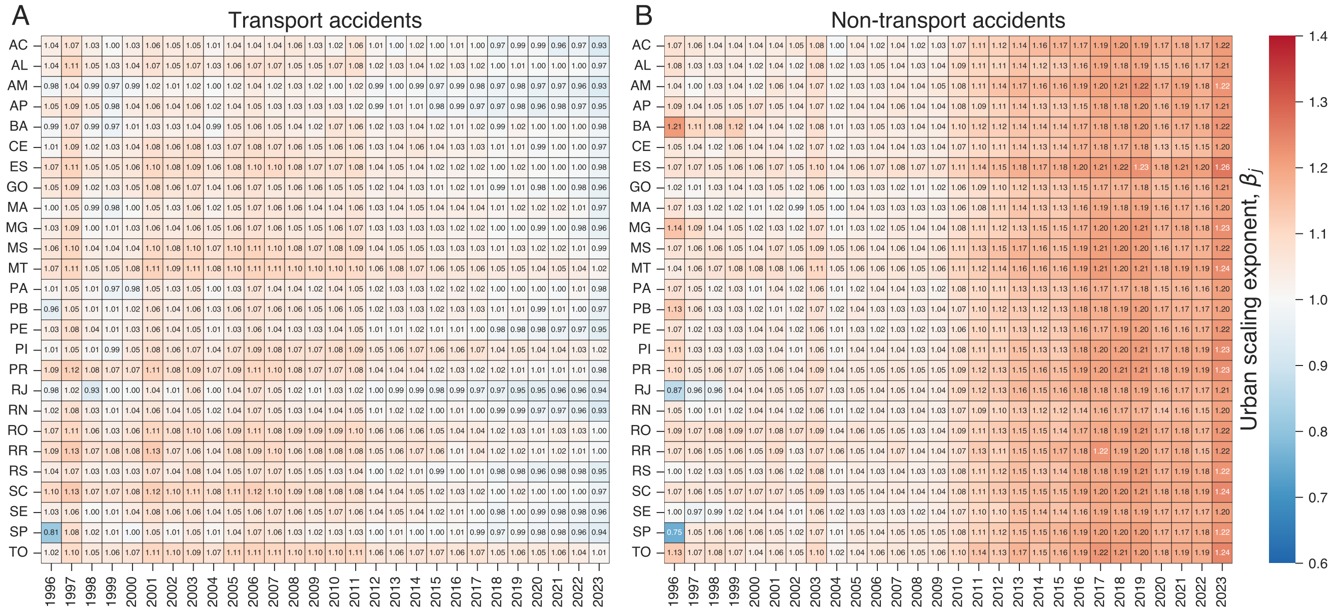

**Figure S12.** Evolution of mortality scaling exponents for transport and non-transport-related accidents in each Brazilian state (1996–2023) quantified by point estimates. Matrix plots display the mean of the posterior distribution of $\beta_j$ over the period for each state. Heatmaps are arranged with rows representing states (denoted by their two-letter abbreviations) and columns corresponding to years. Panels show results for (A) transport accidents and (B) non-transport accidents, using a uniform color scale in which blueish hues indicate sublinear exponents and reddish hues denote superlinear exponents. These visualizations indicate that while the scaling exponents for transport accidents remain approximately stationary over time, they exhibit greater variation across states. In contrast, the exponents for non-transport accidents have shifted toward larger values in line with national trends and display less variation across states.

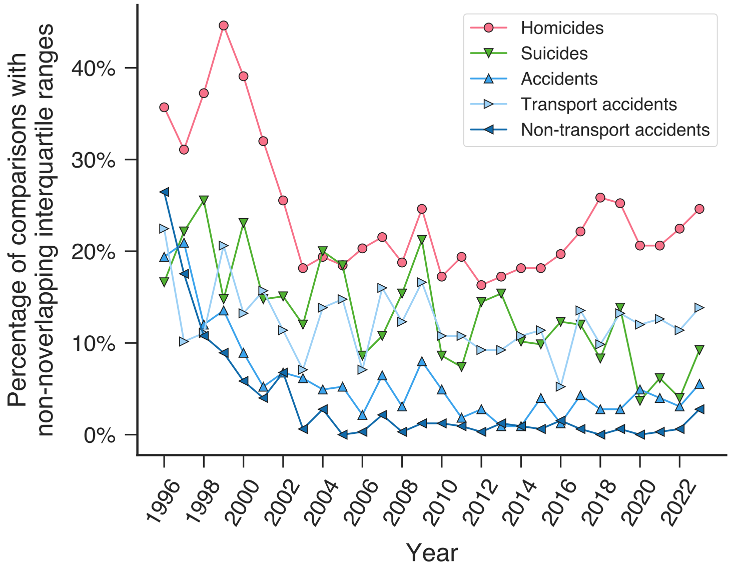


**Figure S13.** Temporal evolution of inter-state variability in scaling exponents, measured as the percentage of pairwise state comparisons with non-overlapping interquartile ranges. Percentage of state pairs with non-overlapping interquartile ranges for homicides, suicides, accidents, transport accidents, and non-transport accidents (as indicated in the legend). Homicides exhibit the highest fraction, followed by suicides and transport accidents, whereas accidents and non-transport accidents show the lowest. These percentages were higher in the late 1990s, declined during the early 2000s, and stabilized after the mid-2000s, indicating a general reduction in inter-state variability in scaling exponents for all external causes of death.

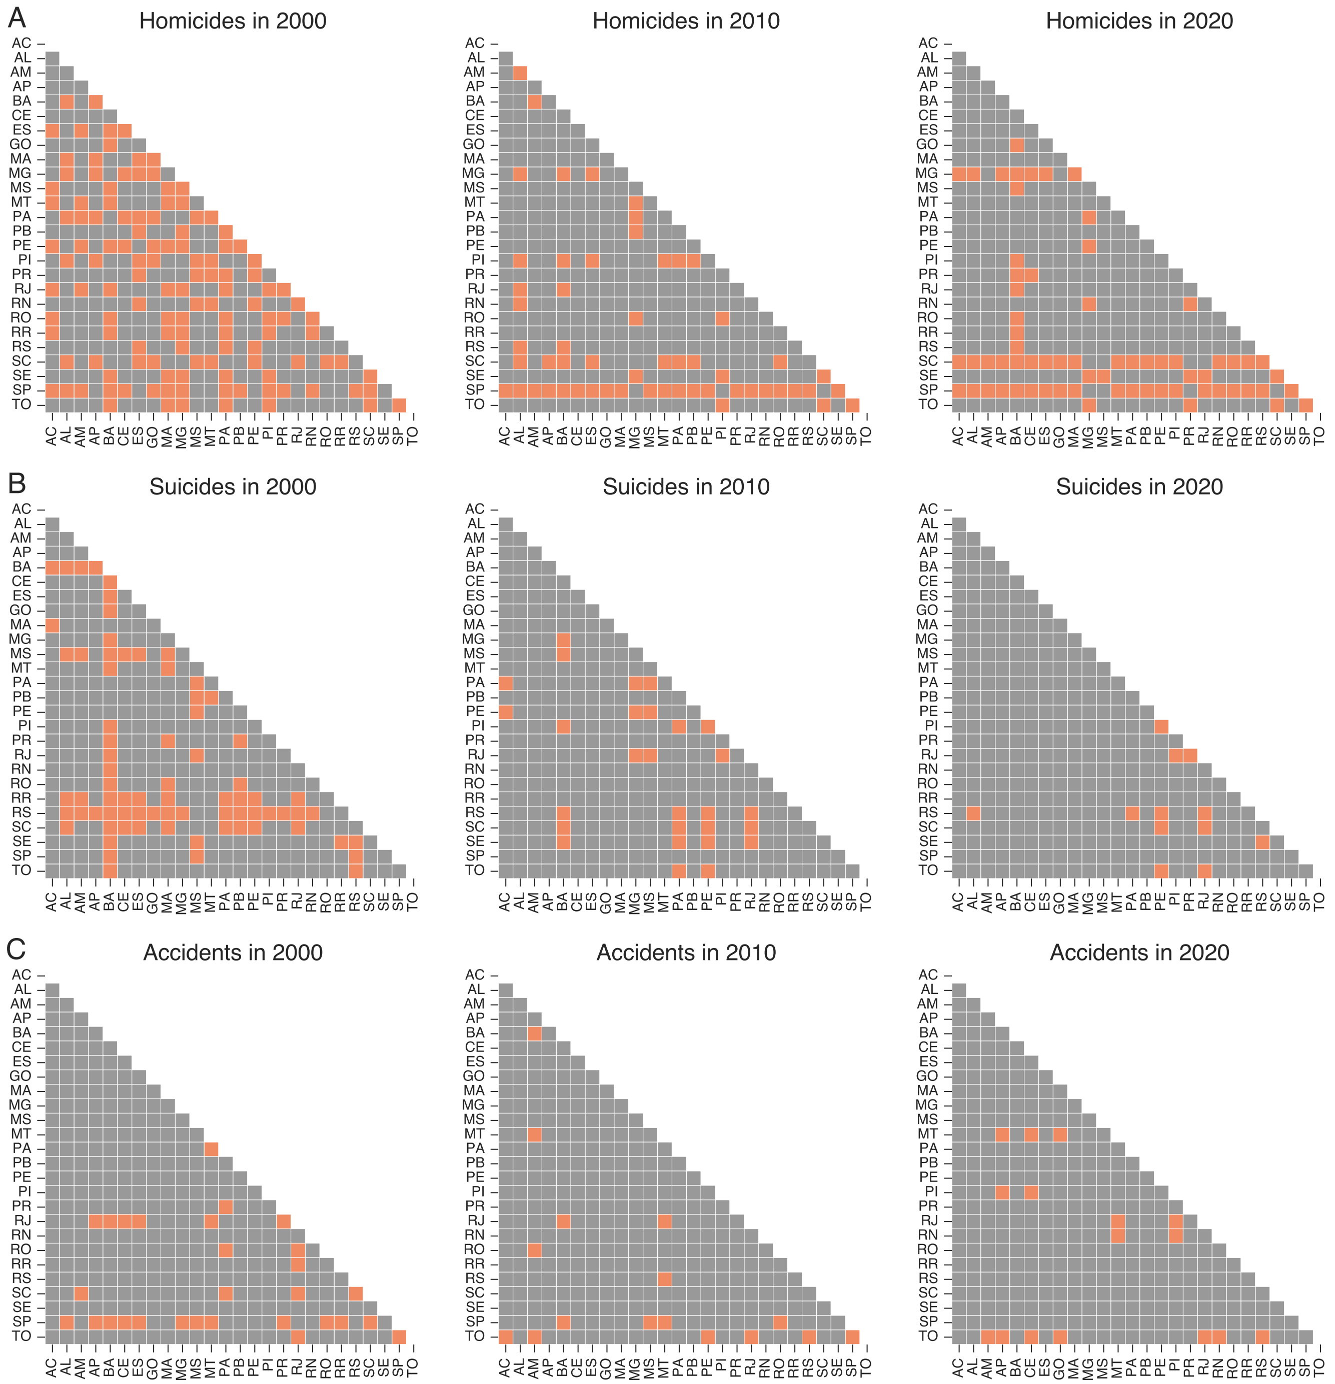


**Figure S14.** Inter-state variability in scaling exponents. Matrix plots depict pairwise comparisons of the posterior distributions of $\beta_j$ across three years (2000, 2010, and 2020, as indicated in the panels) for (A) homicides, (B) suicides, and (C) accidents. Grey cells indicate pairs of states with overlapping interquartile ranges, whereas orange cells denote comparisons with non-overlapping interquartile ranges.

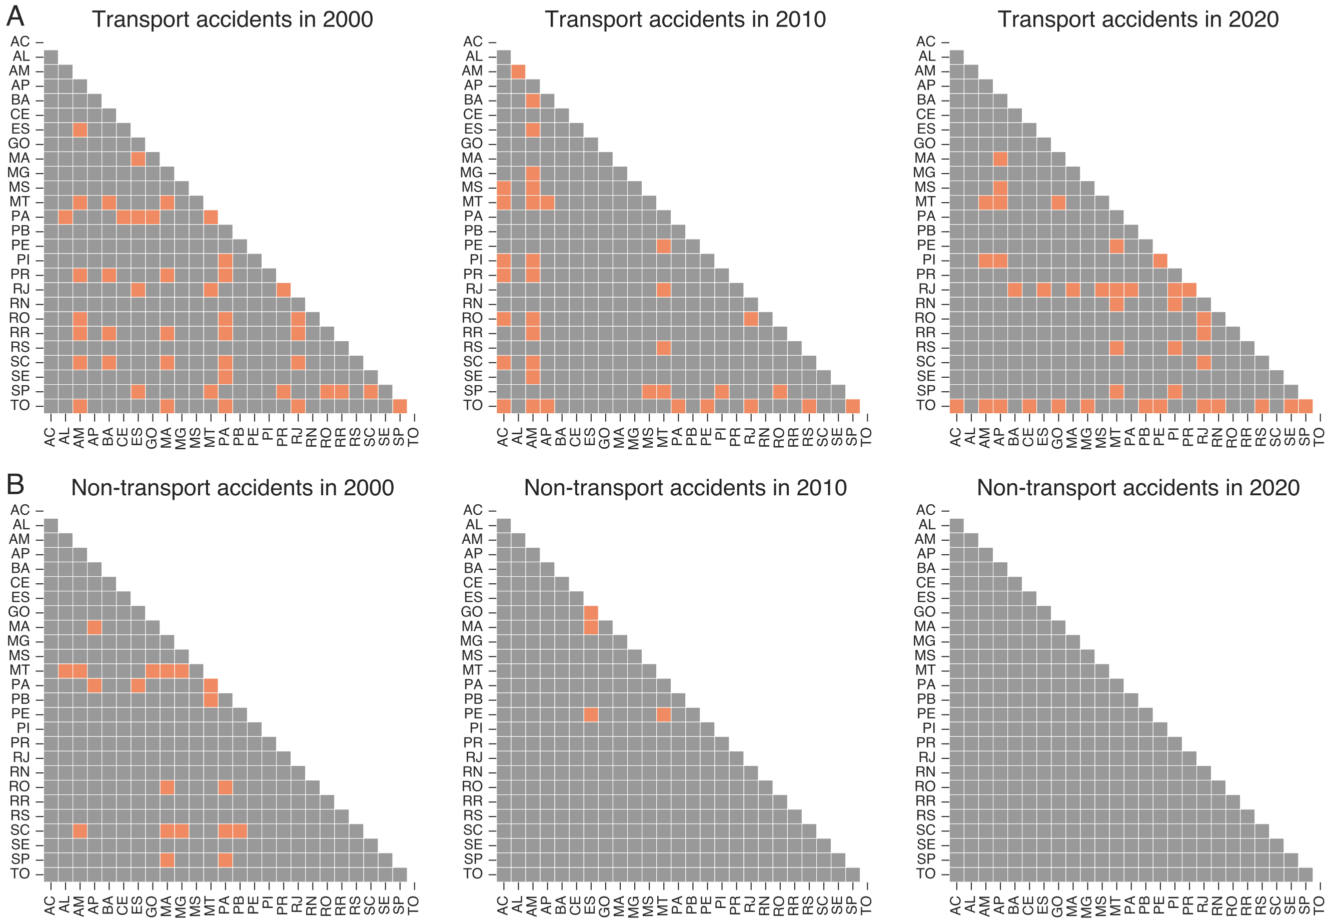


**Figure S15.** Inter-state variability in scaling exponents. Matrix plots depict pairwise comparisons of the posterior distributions of $\beta_j$ across three years (2000, 2010, and 2020, as indicated in the panels) after disaggregating accidents into (A) transport and (B) non-transport categories. Grey cells indicate pairs of states with overlapping interquartile ranges, whereas orange cells denote comparisons with non-overlapping interquartile ranges.

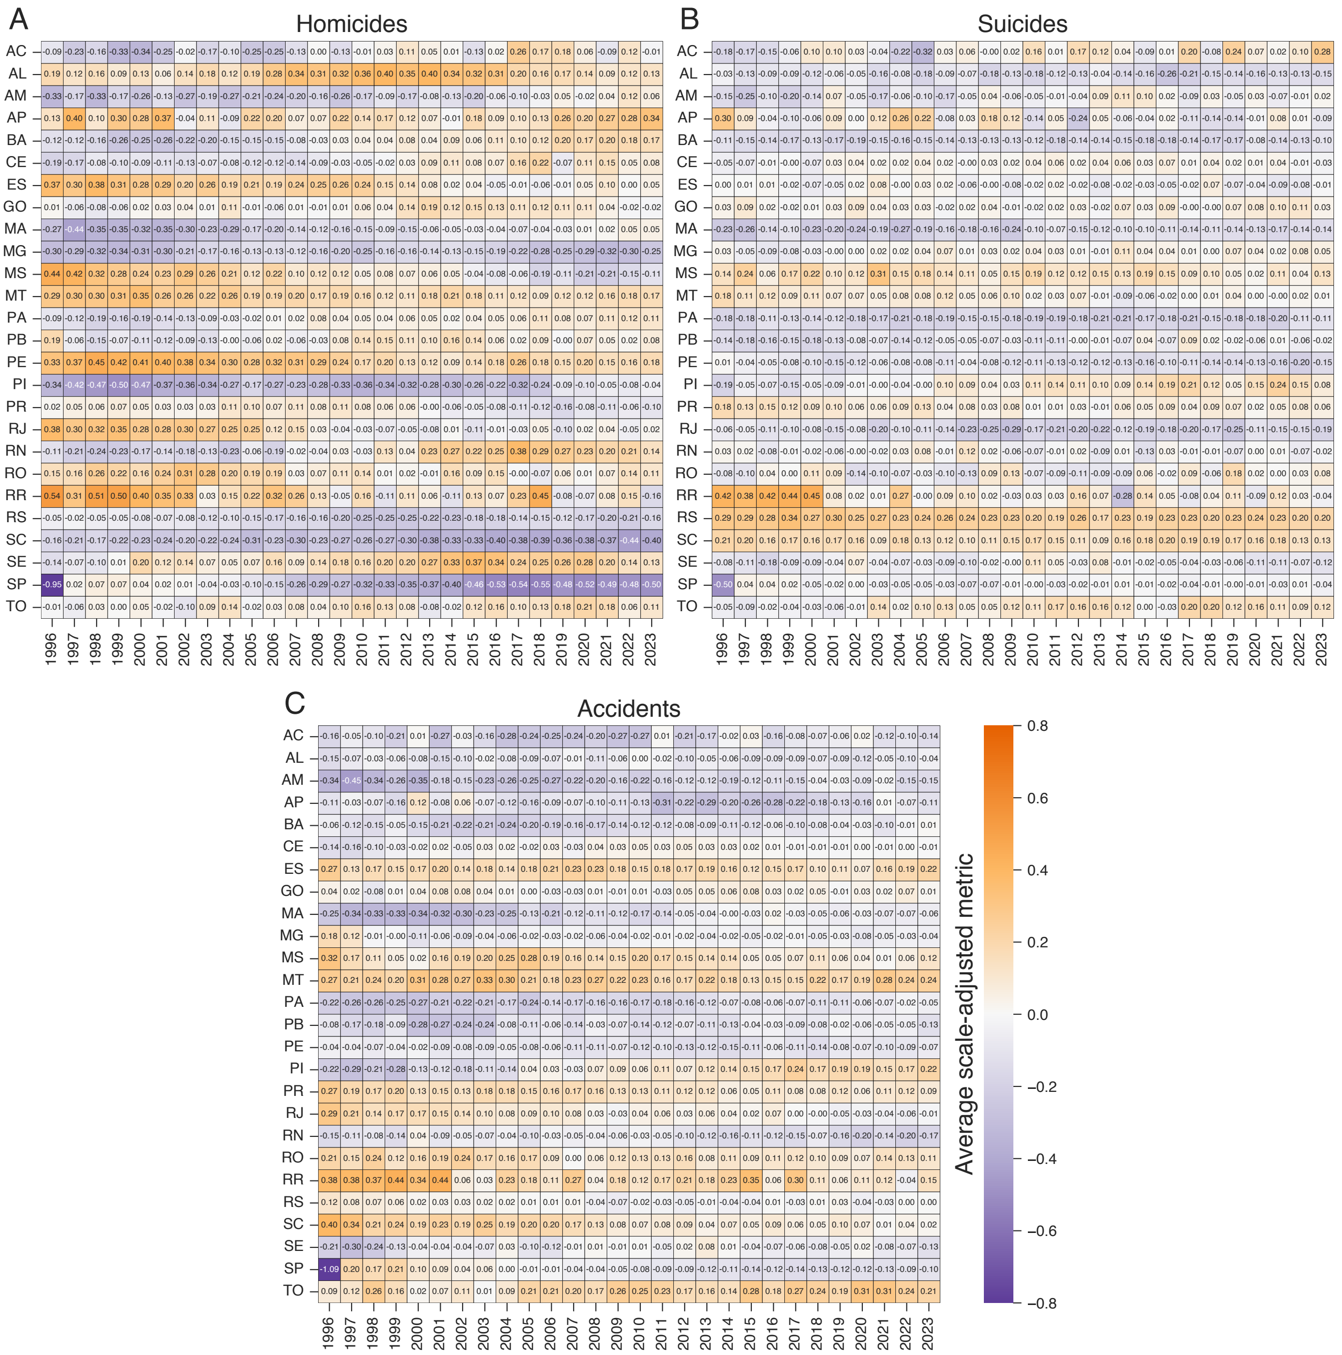


**Figure S16.** Evolution of the mean scale-adjusted metric for each Brazilian state (1996–2023). Matrix plots display the average value of $\xi$ over the period for each state. Heatmaps are arranged with rows representing states (denoted by their two-letter abbreviations) and columns corresponding to years. Panels show results for (A) homicides, (B) suicides, and (C) accidents, using a uniform color scale in which orange tones indicate positive $\xi$ values and purple tones denote negative ones. The trajectories of the average $\xi$ vary across states, with some transitioning from negative to positive or near-zero values (*e.g.* Rio Grande do Norte/RN for homicides and Piauí/PI for accidents), others shifting from positive to negative or near-zero values (*e.g.* Espírito Santo/ES for homicides and Roraima/RR for suicides), and some exhibiting more stable behavior (*e.g.* Rio Grande do Sul/RS for suicides and Minas Gerais/MG for homicides).

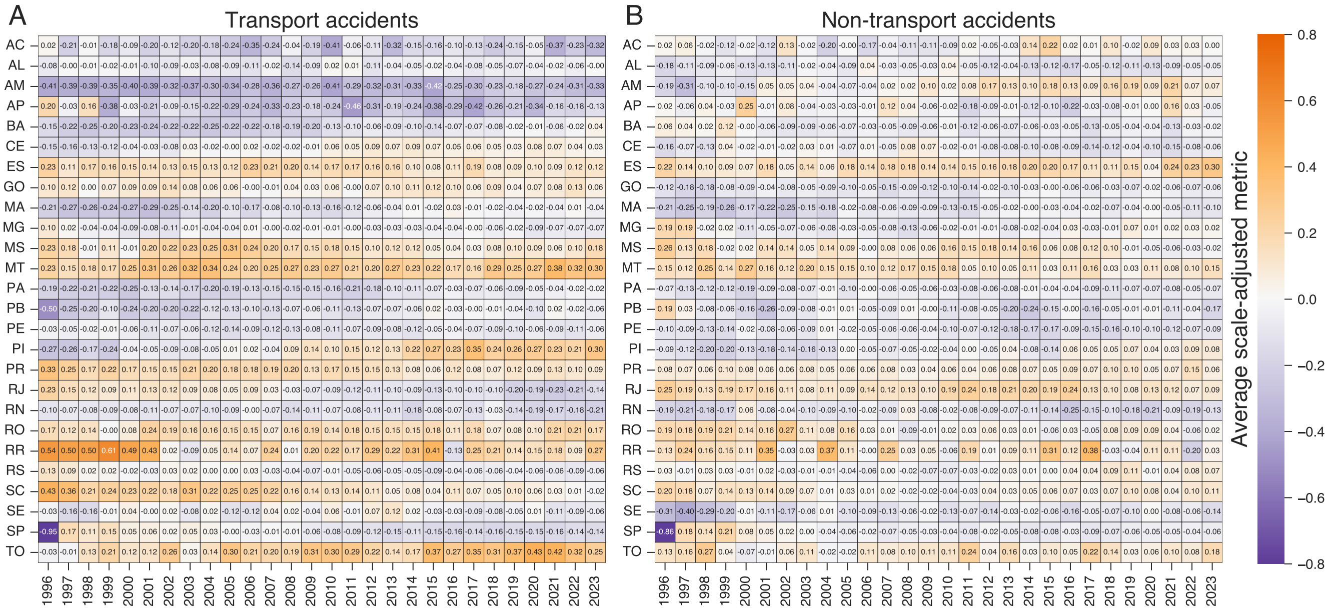


**Figure S17.** Evolution of the mean scale-adjusted metric for transport and non-transport-related accidents in each Brazilian state (1996–2023). Matrix plots display the average value of $\xi$ over the period for each state. Heatmaps are arranged with rows representing states (denoted by their two-letter abbreviations) and columns corresponding to years. Panels show results for (A) transport accidents and (B) non-transport accidents, using a uniform color scale in which orange tones indicate positive $\xi$ values and purple tones denote negative ones. The trajectories of the average $\xi$ vary across states when disaggregating accidents into transport and non-transport categories.

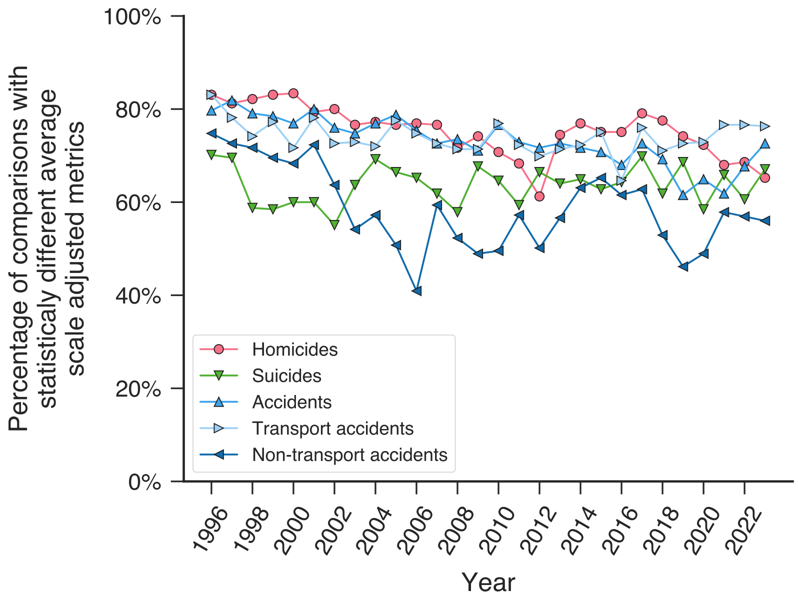


**Figure S18.** Temporal evolution of inter-state variability in the scale-adjusted mortality $\xi$, measured as the percentage of pairwise state comparisons exhibiting statistically significant differences in average $\xi$. The curves represent results for homicides, suicides, accidents, transport accidents, and non-transport accidents (as indicated in the legend). Comparisons were performed using permutation tests at a 95% confidence level, with the Bonferroni correction for multiple comparisons. About two-thirds of all state pairwise comparisons exhibit statistically significant differences.

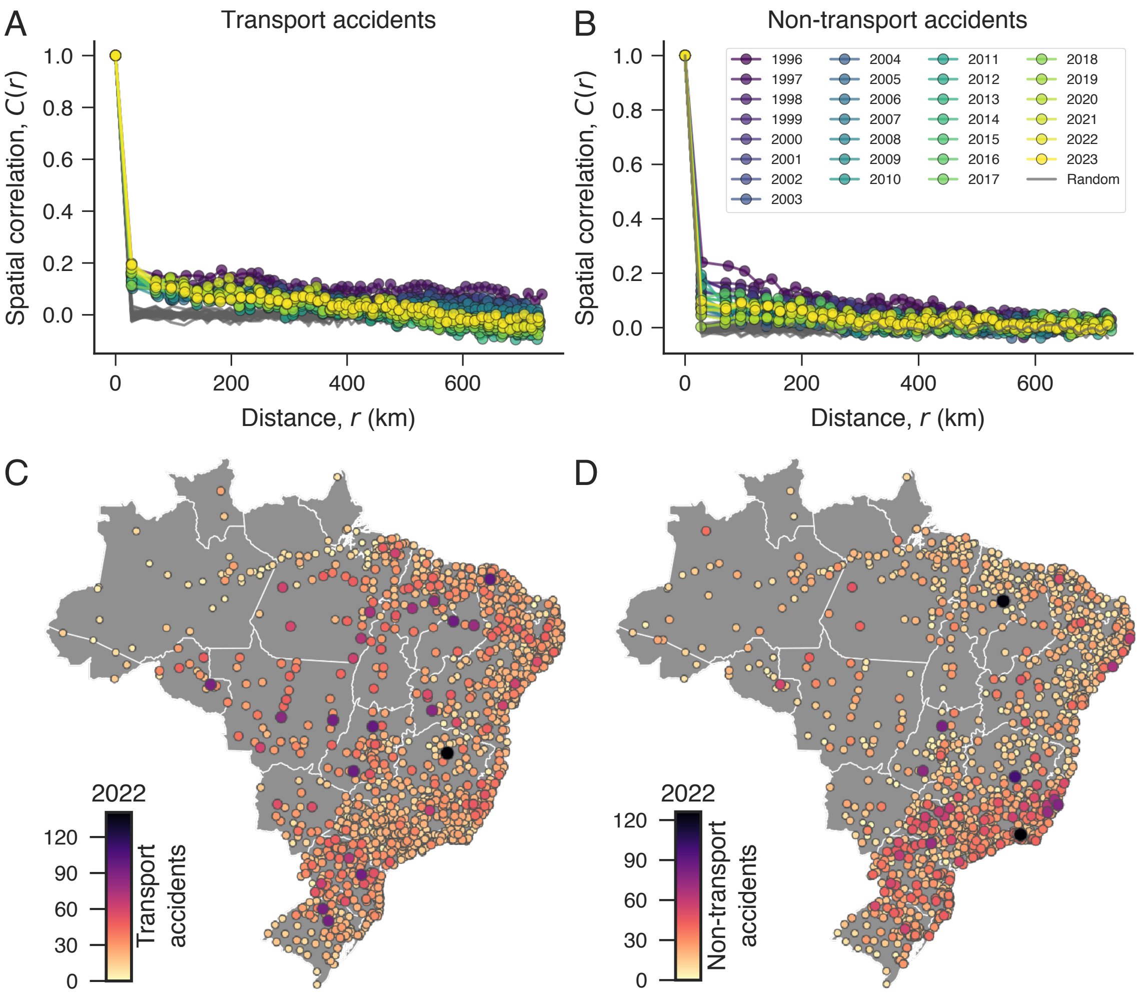


**Figure S19.** Spatial patterns in accident rates disaggregated into transport and non-transport categories. Spatial correlations $C(r)$ of mortality rates as a function of inter-city distance $r$ for (A) transport accidents and (B) non-transport accidents. Colored markers denote specific years (as indicated in the legend), while grey curves represent $C(r)$ values computed after randomly shuffling mortality rates among cities. The value of $C(r)$ corresponds to the Pearson correlation between the mortality rates of all city pairs whose distances fall within a range centered at $r$. Distance ranges are determined based on the percentiles of the inter-city distance distribution, ensuring that each $C(r)$ is estimated from a comparable number of city pairs. Transport accident rates exhibit slightly higher correlations than non-transport accident rates, with the latter closely approaching the randomized baselines. Illustration of the spatial distributions of mortality rates in 2022 for (C) transport accidents and (C) non-transport accidents. In these maps, circles indicate the geographic locations of Brazilian cities, with colors representing mortality rates and marker sizes scaled proportionally to these rates. The maps visually corroborate the correlation analysis, with both accident types exhibiting more uniform spatial distributions than those observed for homicides and suicides.

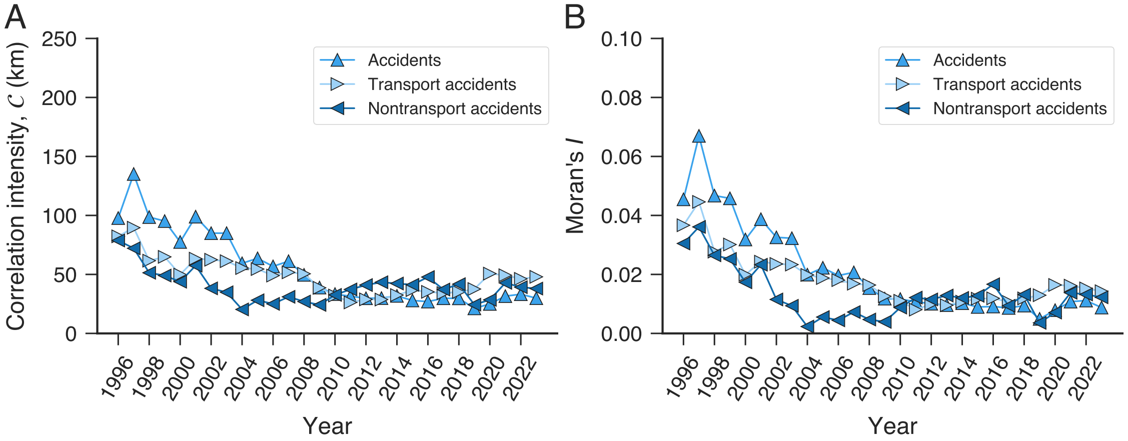


**Figure S20.** Changes in the spatial correlations of accident mortality rates disaggregated into transport and non-transport categories. (A) Evolution of spatial correlation intensity $\mathscr{C}$ and (B) Moran's $I$ spatial correlation coefficient of mortality rates across Brazilian cities for accidents, transport accidents, and non-transport accidents (as indicated in the legend). The values of $\mathscr{C}$, defined as the area under the correlation function, and Moran's $I$ reveal similar trends for accident rates and the disaggregated categories, with no-transport accidents displaying slightly lower values in years before 2010.

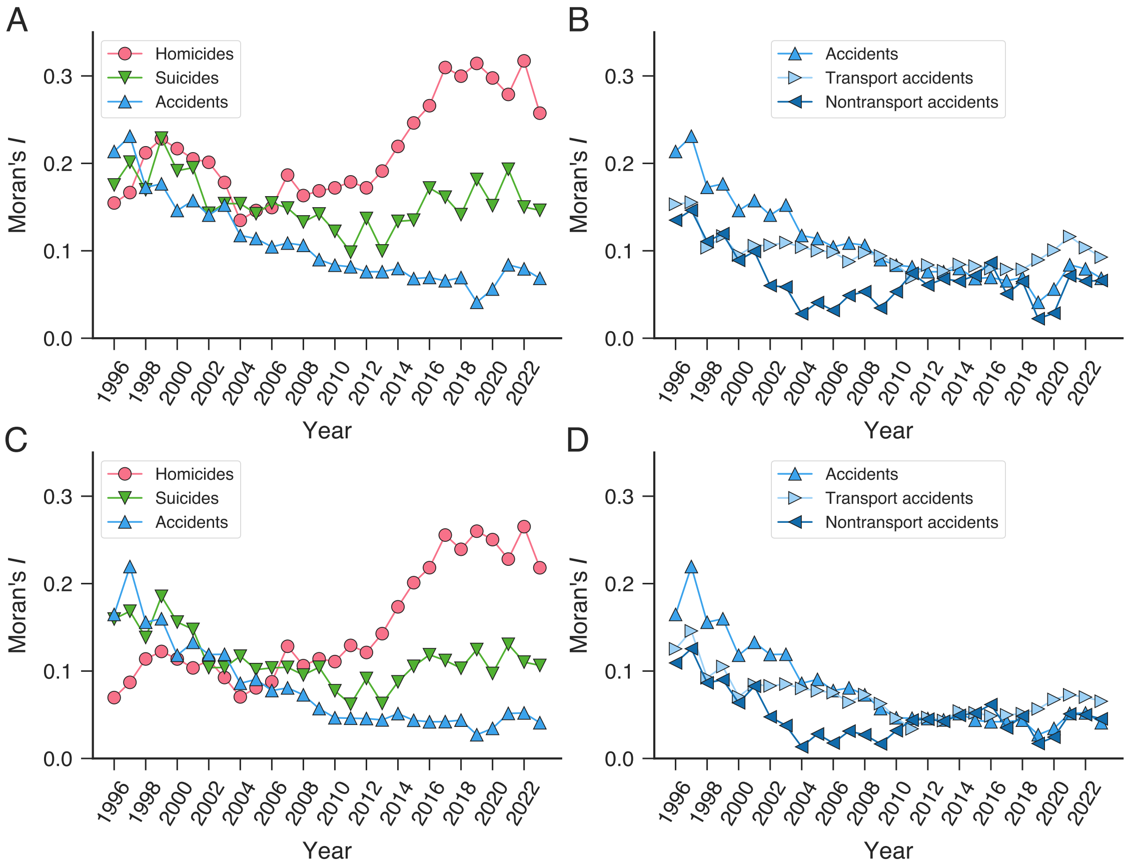


**Figure S21.** Changes in the spatial patterns of mortality rates, as quantified by Moran's $I$ calculated using weights defined by city–neighbor relationships. The weight matrix is defined such that $w_{ij} = 1$ for the first $k$ nearest neighboring cities and $w_{ij} = 0$ otherwise. Panels (A) and (B) show results for $k = 100$, whereas panels (C) and (D) show results for $k = 200$. Panels (A) and (C) display Moran's $I$ for homicides (red circles), suicides (green downward triangles), and accidents (blue upward triangles), while panels (B) and (D) disaggregate accident mortality rates into transport (light blue rightward triangles) and non-transport (dark blue leftward triangles) categories.
